# Supplementary material for: Temperature-dependent rotationally inelastic collisions of OH- and He
Source: arXiv:2010.10061 source file (2020-10-20)
Supplement: Supplementary file 1 [file supplement.pdf]

# Temperature-dependent rotationally inelastic collisions of $OH^-$ and He: Supplementary material

Eric S. Endres[1], Steve Ndengué[2,3], Olga Lakhmanskaya[1], Seunghyun Lee[1], Francesco A. Gianturco[1], Richard Dawes[2], and Roland Wester[1]

[1]*Institut für Ionenphysik und Angewandte Physik, Universität Innsbruck, Technikerstrasse 25/3, 6020 Innsbruck, Austria*

[2]*Department of Chemistry, Missouri University of Science and Technology, 65409 Rolla, Missouri, United States.* and

[3]*ICTP-East African Institute for Fundamental Research, University of Rwanda, Kigali, Rwanda*

(Dated: October 19, 2020)

## $OH^-$+HE SCATTERING

### The two new potential energy surfaces

Two different new PESs were constructed based on interpolation of energies obtained from ab initio electronic structure calculations employing the coupled-cluster (CC) method.

The first PES (denoted $r_0$) fixes the OH bond distance at the diatomic ground state vibrationally averaged distance. It calculated at the level of (AE)-CCSD(T)/CBS, where (AE) indicates that all electrons were included in the correlation treatment, and CBS indicates that the complete basis set limit was estimated by extrapolation. Here the aug-cc-pwCVQZ and aug-cc-pwCV5Z bases[1] (each with an even-tempered extension adding $s$, $p$, $d$ and $f$ functions to the standard basis) were extrapolated using the $l^{-3}$ formula. The OH bond distance was fixed at $r_0$=0.974275 Å, a vibrationally averaged value consistent with the experimental rotational constant of the $OH^-$ anion[2]. A computed correction for the contribution of high-order correlation was also added. The correction was defined as the difference between energies at the CCSDT(Q)/AVTZ and CCSD(T)/AVTZ levels. The MOLPRO[3] and CFOUR[4] electronic structure code packages were used for all of the calculations reported here.

The second PES (denoted $v_0$) was constructed by averaging over the diatomic ground state vibrational probability density. It employs the same level of electronic structure theory as the first PES, but uses separate calculations at a series of OH bond distances in order to average over the diatomic ground state vibrational probability density rather than using a single fixed $r_0$ distance. A variational $J = 0$ vibrational calculation was performed for $OH^-$ using the potential optimized discrete variable representation method[11]. This permits an accurate representation of the lowest vibrational state using just three points located at 0.892135, 1.012750, and 1.146084 Å, with respective weights of 0.334001091, 0.605332536 and 0.060666373. In order to minimize fitting errors, three separate 2D PESs were constructed (one for each of the three necessary bond distances) and then the weights were applied to construct the final vibrationally averaged $v_0$ PES.

Both two-dimensional PESs are represented analytically by interpolating high-level ab initio data using the same interpolating moving least squares (IMLS) method used previously for many vdW systems[5–10]. In this application 475 automatically generated geometries

were determined in the center of mass distance range of $R$=[1.7,15] Å. The fit represents all attractive regions and repulsive regions up to 2800 cm$^{-1}$ above the separate fragments asymptote. A pruned product basis of 39 functions (Legendre and radial) was used for the interpolation. The estimated fitting error with respect to independent test sets is below 0.01 cm$^{-1}$. To represent the long range, an additional 80 points were computed in the range of $R$=[6,25] Å and fit to a Legendre-based analytic representation. A hyperbolic tangent switching function was used to smoothly switch between the short and long range representations. The switch was centered at 9.0 Å making the PES at $R$=9.0 Å a 50:50 mixture of IMLS:long range.

**Properties of the PESs employed in this work**

The global minimum of all three employed PESs is found at a collinear configuration with the He atom at the O-atom end of the $OH^-$ molecule. For the highest level $v_0$ PES, the geometry of the global minimum is $R$=2.691 Å, $\theta$=0$^o$, $E$=-139.21 cm$^{-1}$. For the $r_0$ PES, the geometry of the global minimum is $R$=2.958 Å, $\theta$=0$^o$, $E$=-140.96 cm$^{-1}$. The corresponding data for the earlier PES have been reported in Refs. [12]. Figure 1 shows a plot of the $r_0$ PES in Jacobi coordinates. As seen in Figure 1, a local minimum is found for the other collinear arrangement placing the He atom toward the H-atom. The geometry of the local minimum for the $v_0$ PES is: $R$=3.875 Å, $\theta$=180$^o$, $E$=-38.62 cm$^{-1}$. The geometry of the local minimum for the $r_0$ PES is: $R$=3.809 Å, $\theta$=180$^o$, $E$=-42.13 cm$^{-1}$. The vibrational averaging has a fairly significant impact on the locations of the minima, but a fairly small impact on the well depths.

In order to perform the scattering calculations, the PESs were represented as the radial dependence of a Legendre expansion up to the 8$^{th}$ order according to

$$V(R,\theta) = \sum_{\lambda} v_{\lambda}(R) P_{\lambda}(\theta). \quad (1)$$

The order of the expansion was confirmed to be sufficient by performing convergence test calculations with an expansion order of 10. The first 4 Legendre coefficients for the $r_0$ PES are plotted in Figures 2. In Figure 3 they can be compared to the first 4 Legendre coefficients of the third, earlier PES used in this work, the PES from Gonzalez-Sanchez *et al* [12] that was used in Ref. [13]. We observe from these figures two immediate differences on

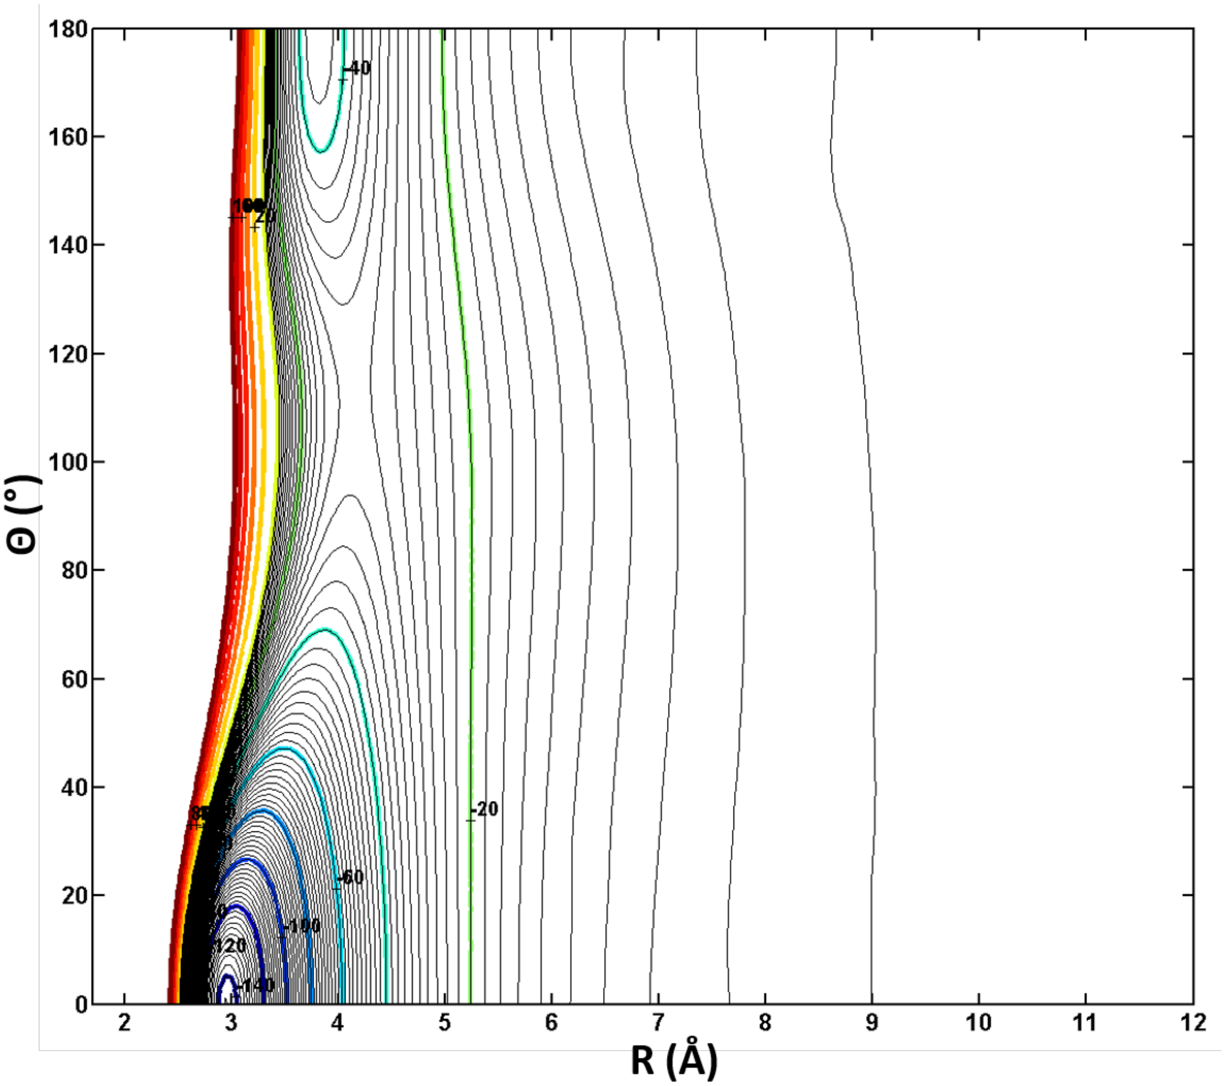


FIG. 1. A plot of the $r_0$ PES. Black contours appear at 2 $cm^{-1}$ intervals and colored contours every 20 $cm^{-1}$.

the even coefficients of the Legendre expansion. While the $l = 2$ term is less deep in the expansion of the new PESs than it is in the same expansion for Gonzalez-Sanchez *et al*'s[12] PES, the opposite is true for the $l = 0$ coefficient. On the other hand, the odd coefficients, those which dominate the action of the dynamical torque causing excitations during the collisions, are very similar in shape and on their repulsive regions. The fact that the $l = 1$ coefficient is slightly more repulsive for the PES of Figure 3 than for that of Figure 2 may well be the cause of finding smaller inelastic cross sections when using the former PES in the calculations.

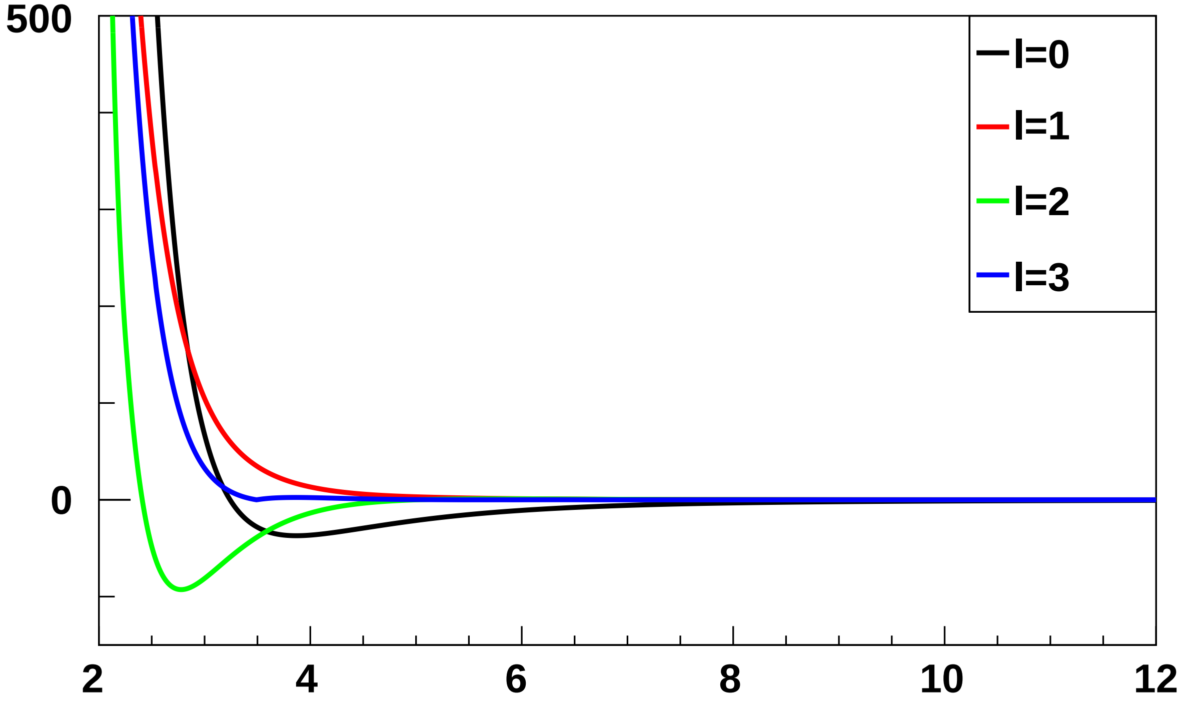


FIG. 2. First 4 Legendre expansion of the $OH^-$-He PES on the $r_0$ PES.

**Scattering Calculations: cross sections and reaction rates**

The scattering theory of a diatomic molecule is well known and documented in the literature. The time independent collisional dynamics calculations where done with the MOLSCAT[14] code. The calculations presented here were performed with the close coupling (CC) method in the full energy range considered. We performed calculations with two different propagators, both yielding the same results: the hybrid modified log-derivative Airy propagator of Alexander and Manolopoulos [15] and the R-matrix propagator of Light and Walker[16]. The results reported here are those from the R-matrix propagator which was found to complete faster at very low energy than the hybrid modified log-derivative Airy propagator.

The $OH^-$ rotational constant[17] used for the calculation is $B_e = 18.5701$ cm$^{-1}$ with the system reduced mass of $\mu = 3.239920422$ AMU. The calculations were done in the $10^{-6}$ – $10^3$ cm$^{-1}$ energy range. The close coupling calculations are done for every total angular momentum value $J_{tot}$ and converged when the last 4 successive $J_{tot}$ values contribute less than 0.0005 and 0.05 Å$^2$ respectively to the inelastic and elastic cross sections. We used an

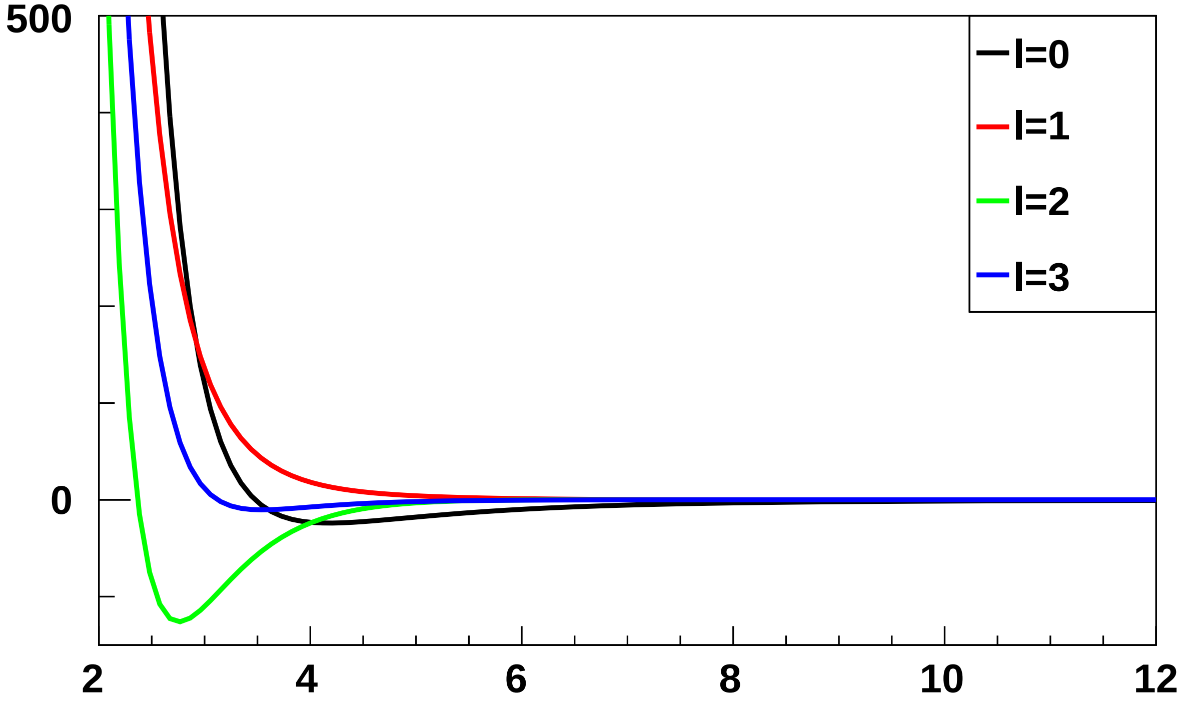


FIG. 3. First 4 Legendre expansion of the $OH^-$-He PES on the Gonzalez-Sanchez *et al*'s[12] PES.

increasing and sufficient number of basis functions to describe the various energy ranges and ensure convergence of the calculations. A maximum of 11 basis functions for the diatomic rotor, which accounts at 1000 $cm^{-1}$ of collisional energy to 7 open states and 4 closed states, were used in the final calculations. The corresponding information pertaining to our earlier PES was given in Ref. [12, 13].

## DENSITY CALIBRATION

The absolute density calbration is carried out as described in the supplementary information of Ref. [13]. The density is calculated using the ideal gas equation from the helium partial pressure measured with a cold cathode gauge in the vacuum chamber. This gauge is calibrated using an accurate capacitive gauge, which can only operate at pressures higher than the low helium partial pressures needed in the present experiment. The pressure is corrected for the gas and chamber temperatures and for the increased particle density inside the cryogenic ion trap compared to the surrounding vacuum chamber. The latter increase is calibrated directly through the comparison with the capacitive gauge that is attached

TABLE I. Error budget of the density

| Variable | Error | comment |
|---|---|---|
| $p$ | 10% | from the reproducibility of the cold cathode gauge |
| $\alpha_{pres}$ | 2.5% | originates from the fluctuations over time which is about the same as the statistical error on the correlation factor |
| $T_T$ | 1% | measured via commercial temperature diodes with a precision below 1% |
| $T_{out}$ | 0.3% | conservative assumption of the room temperature fluctuation on the laboratory |
| $p$ | $\leq 0.04\%$ | systematic error based on the estimation of the residual He background |

directly to the ion trap.

The contributions to the error of the density originate from the pressure measurement $p$, the pressure calibration factor $\alpha_{pres}$, temperature measurement of the trap $T_T$ and the laboratory $T_{out}$. An additional contribution arises from the presence and the fluctuations of residual helium background gas, which yields a systematic error that was estimated using a quadrupole mass spectrometer. All contributions to the error budget of the density are summarized in Table I.


[1] K. A. Peterson and T. H. Dunning Jr, Journal of chemical physics **117**, 10548 (2002).

[2] J. R. Smith, J. B. Kim, and W. C. Lineberger, Phys. Rev. A **55**, 2036 (1997).

[3] H. J. Werner, P. J. Knowles, G. Knizia, F. R. Manby, M. Schütz, *et al.*, "Molpro, version

2012.1, a package of ab initio programs, 2012," (2012).

[4] "See http://www.cfour.de for a description and copy of this software.".

[5] M. Majumder, S. A. Ndengue, and R. Dawes, Molecular Physics **114**, 1 (2016).

[6] R. Dawes, X.-G. Wang, and T. Carrington Jr, Journal of Physical Chemistry A **117**, 7612 (2013).

[7] G. Donoghue, X.-G. Wang, R. Dawes, and T. Carrington, Journal of Molecular Spectroscopy **330**, 170 (2016).

[8] J. Brown, X.-G. Wang, T. Carrington Jr, G. S. Grubbs, and R. Dawes, Journal of chemical physics **140**, 114303 (2014).

[9] X.-G. Wang, T. Carrington, and R. Dawes, Journal of Molecular Spectroscopy **330**, 179 (2016).

[10] K. M. Walker, F. Lique, F. Dumouchel, and R. Dawes, Monthly Notices of the Royal Astronomical Society **466**, 831 (2016).

[11] H. Wei and T. Carrington Jr, Journal of chemical physics **97**, 3029 (1992).

[12] L. Gonzalez-Sanchez, F. Marinetti, E. Bodo, and F. A. Gianturco, J. Phys. B **39**, S1203 (2006).

[13] D. Hauser, S. Lee, F. Carelli, S. Spieler, O. Lakhmanskaya, E. S. Endres, S. S. Kumar, F. Gianturco, and R. Wester, Nat. Phys. **11**, 467 (2015).

[14] J. M. Hutson and S. Green, "Molscat, ver. 14, distributed by collabor. comp. proj. 6, daresbury lab, uk, eng. phys. sci. res. council," (1994).

[15] M. H. Alexander and D. E. Manolopoulos, J. Chem. Phys. **86**, 2044 (1987).

[16] J. C. Light and R. B. Walker, J. Chem. Phys. **65**, 4272 (1976).

[17] J. M. Brown and A. Carrington, *Rotational spectroscopy of diatomic molecules* (Cambridge University Press, 2003).
